# Supplementary material for: Regularized-Likelihood Deconvolution with Posterior-Density Reconstruction
Source: arXiv:2608.00240 source file (2026-09-16)
Supplement: Supplementary file 1 [file supp_xrefs.tex]

% Static cross-reference map generated from the companion document.
% Contains label metadata only; no manuscript content is duplicated.
\makeatletter
\newlabel{supp-app:main-proofs}{{A}{1}}
\newlabel{supp-app:fixed-dimensional-results}{{B}{5}}
\newlabel{supp-app:fixed-model-consistency}{{B.1}{6}}
\newlabel{supp-prop:supp-fixed-consistency}{{S1}{6}}
\newlabel{supp-app:exact-posterior-correction}{{B.2}{6}}
\newlabel{supp-lem:supp-posterior-exact-error}{{S1}{7}}
\newlabel{supp-app:conditional-information-operator}{{B.3}{7}}
\newlabel{supp-lem:supp-conditional-information-operator}{{S2}{7}}
\newlabel{supp-app:ass-primitive-ulln-material}{{C.1}{8}}
\newlabel{supp-prop:gaussian-global-likelihood}{{S2}{8}}
\newlabel{supp-app:observed-norm-conversion}{{C.2}{10}}
\newlabel{supp-lem:supp-kl-to-l2}{{S3}{10}}
\newlabel{supp-app:global-shrinking-scale}{{C.3}{10}}
\newlabel{supp-prop:supp-obs-scale-appr}{{S3}{10}}
\newlabel{supp-prop:supp-self-contained-en}{{S4}{11}}
\newlabel{supp-app:gaussian-localization-tools}{{C.4}{11}}
\newlabel{supp-lem:marginal-log-moment}{{S4}{11}}
\newlabel{supp-lem:penalized-likelihood-localization}{{S5}{11}}
\newlabel{supp-app:gaussian-fixed-scale-hellinger}{{C.5}{12}}
\newlabel{supp-lem:gaussian-fixed-scale-hellinger}{{S6}{12}}
\newlabel{supp-app:gaussian-fixed-scale-observed-rates}{{C.6}{13}}
\newlabel{supp-prop:supp-gaussian-smoothed-klv-approximation}{{S5}{13}}
\newlabel{supp-eq:gaussian-smoothed-kl-approximation}{{S1}{13}}
\newlabel{supp-eq:gaussian-klv-approximation}{{S2}{13}}
\newlabel{supp-prop:supp-gaussian-smoothed-observed-rate}{{S6}{15}}
\newlabel{supp-app:gaussian-fixed-scale-inverse-posterior}{{C.7}{16}}
\newlabel{supp-lem:supp-gaussian-analytic-stability}{{S7}{16}}
\newlabel{supp-lem:supp-gaussian-smoothed-l1-transfer}{{S8}{17}}
\newlabel{supp-lem:supp-gaussian-posterior-lipschitz}{{S9}{17}}
\newlabel{supp-prop:supp-gaussian-smoothed-posterior-complexity}{{S7}{17}}
\newlabel{supp-app:posterior-truncation-material}{{C.8}{18}}
\newlabel{supp-lem:explicit-mn}{{S10}{18}}
\newlabel{supp-cor:explicit-mn-laplace}{{S1}{18}}
\newlabel{supp-cor:explicit-mn-gaussian}{{S2}{19}}
\newlabel{supp-app:fourier-inverse-material}{{C.9}{19}}
\newlabel{supp-cor:supp-generic-supersmooth-transfer}{{S3}{19}}
\newlabel{supp-lem:gaussian-sieve-budgets}{{S11}{20}}
\newlabel{supp-lem:supp-bias-separated-inverse}{{S12}{20}}
\newlabel{supp-app:localized-ordinary-rate-material}{{C.10}{21}}
\newlabel{supp-prop:supp-local-observed-rate}{{S8}{21}}
\newlabel{supp-lem:supp-local-direct-inverse}{{S13}{21}}
\newlabel{supp-lem:supp-local-l2-l1}{{S14}{22}}
\newlabel{supp-app:laplace-ordinary-verification}{{C.11}{22}}
\newlabel{supp-prop:supp-concrete-laplace-ap}{{S9}{22}}
\newlabel{supp-eq:concrete-ap}{{S3}{22}}
\newlabel{supp-prop:supp-concrete-laplace-ll}{{S10}{24}}
\newlabel{supp-eq:concrete-laplace-hellinger-entropy}{{S4}{24}}
\newlabel{supp-prop:supp-concrete-laplace-pe}{{S11}{25}}
\newlabel{supp-eq:concrete-pe}{{S5}{25}}
\newlabel{supp-app:posterior-stability-gaussian}{{C.12}{25}}
\newlabel{supp-lem:posterior-kernel-lipschitz}{{S15}{25}}
\newlabel{supp-lem:posterior-kernel-bracketing}{{S16}{26}}
\newlabel{supp-prop:posterior-stability-gaussian}{{S12}{27}}
\newlabel{supp-proof:prop-posterior-stability-gaussian}{{C.12}{27}}
\newlabel{supp-app:fitted-denominator-material}{{C.13}{28}}
\newlabel{supp-tab:tail-verification}{{S1}{28}}
\newlabel{supp-app:post-stability-calibration}{{C.14}{29}}
\newlabel{supp-app:fixed-order-selection}{{C.15}{29}}
\newlabel{supp-prop:fixed-order-selection}{{S13}{29}}
\newlabel{supp-cor:fixed-order-gaussian}{{S4}{30}}
\newlabel{supp-cor:fixed-order-laplace}{{S5}{30}}
\newlabel{supp-lem:laplace-component-comparison}{{S17}{31}}
\newlabel{supp-lem:laplace-posterior-envelope}{{S18}{32}}
\newlabel{supp-lem:laplace-posterior-covering}{{S19}{32}}
\newlabel{supp-supp_EMoptim}{{D}{33}}
\newlabel{supp-cor:em-error}{{S6}{33}}
\newlabel{supp-app:laplace-posterior-moments}{{E}{34}}
\newlabel{supp-sec:numerical-safeguards}{{F}{34}}
\newlabel{supp-tab:numerical-safeguards}{{S2}{34}}
\newlabel{supp-app:selected-k-details}{{G}{36}}
\newlabel{supp-tab:selected-k-by-latent-n}{{S3}{36}}
\newlabel{supp-app:complete-simulation-table}{{H}{36}}
\newlabel{supp-tab:symmetric-unimodal-mise-se}{{S4}{36}}
\newlabel{supp-tab:asymmetric-unimodal-gaussian-sieve-mise-se}{{S5}{38}}
\newlabel{supp-tab:skew-asym-full}{{S6}{39}}
\newlabel{supp-tab:bimodal-mise-se}{{S7}{41}}
\newlabel{supp-tab:pairwise-all-expanded}{{S8}{42}}
\@ifundefined{r@supp-prop:supp-fixed-consistency}{}{%
  \expandafter\let\csname r@supp-prop\expandafter\endcsname\csname r@supp-prop:supp-fixed-consistency\endcsname
}
\makeatother
